# Supplementary material for: Doping: A technique for efficient compression of LSTM models using sparse structured additive matrices
Source: arXiv:2102.07071 source file (2021-02-14)
Supplement: Supplementary file 2 [file OtherStructures.tex]

\section{Compatibility of Doping with other structures}
\label{sec:otherStruct}
\subsection{Compatibility of doping with other fixed structures}
Doping is applicable to other structures apart from Kronecker. To verify this, we dope on top of a matrix factorized to a lower-rank (LMF), creating a new compression technique called Doped LMF. The results of compressing using Doped LMF vs doing traditional LMF can be found in Table \ref{tab:dopedlmf}. As shown in the table, for iso-compression points, doped LMF outperforms traditional LMF by a large margin. 

\begin{table}[htb]
\begin{tabular}{lccc}
\toprule
Baseline & \multicolumn{3}{c}{82.1} \\
\midrule
Compression Factor & 30x & 25x & 20x \\
\midrule
\begin{tabular}[c]{@{}l@{}}Low-rank factorization \\ (LMF)\end{tabular} & 110.1 & 108.6 & 103.4 \\
Doped LMF & 90.8 & 89.6 & 89.2 \\
\bottomrule
\end{tabular}
\caption{Test  perplexity  after  compressing  medium LM in \cite{ptblm}  over  multiple  compression  factors  using traditional low-rank matrix factorization (LMF) and Doped LMF. Doped LMF achieves far better test accuracy than traditional LMF showing the general applicability of doping technique for structured matrices.}
\label{tab:dopedlmf}
\end{table}
