# Supplementary material for: Doping: A technique for efficient compression of LSTM models using sparse structured additive matrices
Source: arXiv:2102.07071 source file (2021-02-14)
Supplement: Supplementary file 3 [file SmallLarge.tex]

\section{Other benchmarks compressed}
\label{sec:appendresults}
% Please add the following required packages to your document preamble:
% \usepackage{booktabs}
\begin{table}[h]
\begin{tabular}{@{}lcc@{}}
\toprule
\begin{tabular}[c]{@{}l@{}}Comparison\\with Prior Art\end{tabular} & \begin{tabular}[c]{@{}l@{}}Compression \\ Factor\end{tabular} & \begin{tabular}[c]{@{}l@{}}Test \\ ppl\end{tabular} \\
\midrule
Baseline & $1\times$ & 115.9 \\
\cite{2017_c1} & $8\times$ & 114.9 \\
\cite{2018_c2} & $10.67\times$ & 116.6 \\
LMF & $20\times$ & 137.9 \\
Pruning & $20\times$ & 113.7 \\
Ours & $20\times$ & 108.2 \\ 
\bottomrule
\end{tabular}
\caption{Comparing DKP with previous published work targeting the small LM in \cite{ptblm}}
\label{tab:ptbsmall}
\end{table}

\iffalse
\begin{table}[h]
\begin{tabular}{@{}lcc@{}}
\toprule
\begin{tabular}[c]{@{}l@{}}Comparison\\with Prior Art\end{tabular} & \begin{tabular}[c]{@{}l@{}}Compression \\ Factor\end{tabular} & \begin{tabular}[c]{@{}l@{}}Test \\ ppl\end{tabular} \\
\midrule
Baseline & $1\times$ & 78.3 \\
\cite{2017_c1} & $8\times$ & 78.1 \\
\cite{iss} & $9.83\times$ & 78.6 \\
\cite{DBLP:journals/corr/abs-1906-06847} & $10.71\times$ & 78.1 \\
\cite{lobacheva2019structured} & $3.22\times$ & 77.8 \\
Pruning & $25\times$ &  83.4\\
Ours & $25\times$ & 79.3 \\
\bottomrule
\end{tabular}
\caption{Comparing DKP with previous published work targeting the large LM in \cite{ptblm}}
\label{tab:ptblarge}
\end{table}
\fi
